# Supplementary material for: Strategic Multi-Armed Bandit Problems Under Debt-Free Reporting
Source: arXiv:2501.16018 source file (2025-01-27)
Supplement: Supplementary file 1 [file local_aliases.tex]

\usepackage{thmtools}
\usepackage{thm-restate}
\usepackage{enumitem}
\usepackage{parskip}
\usepackage{dsfont}
\usepackage{lipsum}                     
\usepackage{xargs}  


%%%%%%%%%%%%%%%%%%%%%%%%%%%%%%%%%%%%%%
\newcommand\norm[1]{\lVert#1\rVert}
\newcommand\normx[1]{\Vert#1\Vert}
\newcommand\abs[1]{\left\lvert#1\right\rvert}
\newcommand\Det[1]{\det\left(#1\right)}
\newcommand\Log[1]{\log\left(#1\right)}
\newcommand\vol[1]{\text{vol}\left(#1\right)}
%%%%%%%%%%%%%%%%%%%%%%%%%%%%%%%%%%


\newcommand{\cA}{\mathcal{A}}
\newcommand{\cB}{\mathcal{B}}
\newcommand{\cC}{\mathcal{C}}
\newcommand{\cD}{\mathcal{D}}
\newcommand{\cE}{\mathcal{E}}
\newcommand{\cF}{\mathcal{F}}
\newcommand{\cG}{\mathcal{G}}
\newcommand{\cH}{\mathcal{H}}
\newcommand{\cI}{\mathcal{I}}
\newcommand{\cJ}{\mathcal{J}}
\newcommand{\cK}{\mathcal{K}}
\newcommand{\cL}{\mathcal{L}}
\newcommand{\cM}{\mathcal{M}}
\newcommand{\cN}{\mathcal{N}}
\newcommand{\cO}{\mathcal{O}}
\newcommand{\co}{\mathcal{o}}
\newcommand{\cP}{\mathcal{P}}
\newcommand{\cQ}{\mathcal{Q}}
\newcommand{\cR}{\mathcal{R}}
\newcommand{\cS}{\mathcal{S}}
\newcommand{\cT}{\mathcal{T}}
\newcommand{\cU}{\mathcal{U}}
\newcommand{\cV}{\mathcal{V}}
\newcommand{\cW}{\mathcal{W}}
\newcommand{\cX}{\mathcal{X}}
\newcommand{\cY}{\mathcal{Y}}
\newcommand{\cZ}{\mathcal{Z}}

\newcommand{\bA}{\mathbf{A}}
\newcommand{\bB}{\mathbf{B}}
\newcommand{\bC}{\mathbf{C}}
\newcommand{\bD}{\mathbf{D}}
\newcommand{\bE}{\mathbf{E}}
\newcommand{\bF}{\mathbf{F}}
\newcommand{\bG}{\mathbf{G}}
\newcommand{\bH}{\mathbf{H}}
\newcommand{\bI}{\mathbf{I}}
\newcommand{\bJ}{\mathbf{J}}
\newcommand{\bK}{\mathbf{K}}
\newcommand{\bL}{\mathbf{L}}
\newcommand{\bM}{\mathbf{M}}
\newcommand{\bN}{\mathbf{N}}
\newcommand{\bO}{\mathbf{O}}
\newcommand{\bP}{\mathbf{P}}
\newcommand{\bQ}{\mathbf{Q}}
\newcommand{\bR}{\mathbf{R}}

\newcommand{\bzeta}{\boldsymbol{\zeta}}
\newcommand{\bb}{\mathbf{b}}
\newcommand{\bm}{\mathbf{m}}
\newcommand{\bo}{\mathbf{o}}
\newcommand{\bp}{\mathbf{p}}
\newcommand{\bq}{\mathbf{q}}
\newcommand{\bs}{\mathbf{s}}
\newcommand{\by}{\mathbf{y}}
\newcommand{\bz}{\mathbf{z}}

\newcommand{\s}{\xvector s}


\newcommand{\lE}{\mathbb{E}}
\newcommand{\lN}{\mathbb{N}}
\newcommand{\lP}{\mathbb{P}}
\newcommand{\lV}{\mathbb{V}}
\newcommand{\lR}{\mathbb{R}}



\newcommand{\indicator}[1]{{\mathds{1}_{\left[#1\right]}}}
\newcommand{\Setindicator}[1]{{\underline{\mathds{1}}_{\left[#1\right]}}}
\newcommand{\intset}[1]{{[\![#1]\!]}}
\newcommand{\sminus}{\text{-}}
\newcommand{\dotprod}[2]{{\langle#1,#2\rangle}}
\newcommand{\tendsto}[1]{\xrightarrow[#1]{}}



\newcommand{\ahmed}[1]{\textcolor{green}{ABY: #1}}
\newcommand{\clem}[1]{\textcolor{orange}{CC: #1}}
\newcommand{\vianney}[1]{\textcolor{purple}{VP: #1}}






\usepackage{dsfont}


\def\stackbelow#1#2{\underset{\displaystyle\overset{\displaystyle\shortparallel}{#2}}{#1}}

\def\stackover#1#2{\overset{\displaystyle\overset{\displaystyle\shortparallel}{#2}}{#1}}

\DeclareMathOperator*{\argmin}{argmin}
\DeclareMathOperator*{\argmax}{argmax}

\def\stackbelow#1#2{\underset{\displaystyle\overset{\displaystyle\shortparallel}{#2}}{#1}}
